# Supplementary material for: KiDS-1000 Cosmology: Cosmic shear constraints and comparison between two point statistics
Source: arXiv:2007.15633 source file (2020-10-13)
Supplement: Supplementary file 1 [file appendixG.tex]

\label{app:constraint_changes}

Let $X\sim N(0,\sigma^2)$, $Y\sim N(0,\sigma^2)$, and $Z=\frac{1}{2}(X+Y)$ with $Z\sim N(0, \frac{1}{2}\sigma^2)$. Think $X$=`KV450' and $Z$=`KiDS-1000'.

Now consider $\Delta=Z-X$, i.e., the difference between the `KiDS-1000' and `KV450'. We have $\Delta=\frac{1}{2}(Y-X)$, i.e., $\Delta\sim N(0, \frac{1}{2}\sigma^2)$.

The absolute difference ($|\Delta|$) is distributed as a folded Gaussian, with mean $\mathrm{E}[|\Delta|] = \sqrt{\frac{2}{\pi}}\sigma_\Delta = \sqrt{\frac{1}{\pi}}\sigma$, and CDF
\begin{equation}
   \mathrm{CDF}(x) = \mathrm{erf}\left(\frac{x}{\sigma_\Delta\sqrt{2}}\right) = \mathrm{erf}\left(\frac{x}{\sigma}\right) \ .
\end{equation}

Putting in numbers, the expected (absolute) offset between $X$ and $Z$ is $\approx 0.5\sigma$. There is a 16\% chance of getting offsets larger than $1\sigma$.

\paragraph{Improved treatment}
Since the m-calibration for KiDS-1000 is improved, the uncertainty of KiDS-1000 on the KV450 footprint is reduced. This can be modelled as $(X_1, X_2, Y)\sim N(0,\Sigma)$, where
\begin{equation}
  \Sigma = \begin{pmatrix}
              \sigma_1^2       & \sigma_1\sigma_2 & 0\\
              \sigma_1\sigma_2 & \sigma_2^2       & 0\\
              0                & 0                & \sigma_2^2
            \end{pmatrix}\, ,
\end{equation}
where $\sigma_1$ is the `KV450' uncertainty and $\sigma_2$ is the `KiDS-1000' uncertainty on the `KV450' footprint. On the `KV450' footprint the measurements $X_1$ and $X_2$ are 100\% correlated. 
Now, let $Z = \frac{1}{2}(X_2+Y)$ be the KiDS-1000' measurement and $\Delta = Z - X_1$ the offset between the `KiDS-1000' and `KV450' measurements. We have $\sigma_\Delta^2 = \mathrm{Var}[\Delta] = \sigma_1^2 + \frac{\sigma_2^2}{2} - \sigma_1\sigma_2$. The expectation and CDF for $|\Delta|$ follows as above.
